# Supplementary material for: Stop Looking for Important Tokens in Multimodal Language Models: Duplication Matters More
Source: arXiv:2502.11494 source file (2025-06-08)
Supplement: Supplementary file 1 [file appendix_qwen2vl.tex]

\begin{table*}[!h]
    \centering
    \resizebox{0.75\textwidth}{!}{\setlength{\tabcolsep}{3pt}
    
    {\begin{tabular}{p{2.5cm} | c c c c c c c | >{\centering\arraybackslash}p{1.2cm}}
        \toprule[1.5pt]
        \textbf{Method} & \textbf{GQA} & \textbf{MMB} & \textbf{MMB-CN} & \textbf{MME} & \textbf{POPE} & \textbf{SQA} & \textbf{VQA}$^{\text{Text}}$ & \makecell[c]{\textbf{Avg}.}\\
        \hline
        \rowcolor{mygray}
        Qwen2-VL-7B & \multicolumn{8}{c}{\textit{Upper Bound, All Tokens} \ $\textbf{(100\%)}$}   \\
        \textcolor{gray}{Vanilla} & \textcolor{gray}{62.2} & \textcolor{gray}{80.5} & \textcolor{gray}{81.2} & \textcolor{gray}{2317} & \textcolor{gray}{86.1} & \textcolor{gray}{84.7} & \textcolor{gray}{82.1} & \multirow{1}*{\textcolor{gray}{100\%}} \\
        \hline

        \rowcolor{mygray}
        Qwen2-VL-7B & \multicolumn{8}{c}{\textit{Token Reduction} \ $\fg{(\downarrow 66.7\%)}$}   \\
        \hspace{0.2em} + FastV \texttt{\scriptsize{(ECCV24)}} & - & - & - & - & - & - & - & -  \\
        \hspace{0.2em} + \algname (Ours) & 61.6 & 80.7 & 81.0 & 2344 & 85.6 & 84.1 & 82.2 & -  \\
        \hline

        \rowcolor{mygray}
        Qwen2-VL-7B & \multicolumn{8}{c}{\textit{Token Reduction} \ $\fg{(\downarrow 77.8\%)}$}\\
        \hspace{0.2em} + \multirow{1}*{FastV \texttt{\scriptsize{(ECCV24)}}} & - & - & - & - & - & - & - & -  \\
        \hspace{0.2em} + \algname (Ours) & 61.7 & 80.6 & 81.0 & 2319 & 85.6 & 84.0 & 82.1 & -  \\
        \hline

        \rowcolor{mygray}
        Qwen2-VL-7B & \multicolumn{8}{c}{\textit{Token Reduction} \ $\fg{(\downarrow 88.9\%)}$}\\
        \hspace{0.2em} + \multirow{1}*{FastV \texttt{\scriptsize{(ECCV24)}}} & - & - & - & - & - & - & - & -  \\
        \hspace{0.2em} + \algname (Ours) & 61.7 & 80.3 & 81.0 & 2311 & 85.1 & 83.7 & 82.0 & -  \\

        \bottomrule[1.5pt]
	\end{tabular}}}
	\caption{\textbf{Comparative Experiments on Qwen2-VL-7B}. Note: Qwen2-VL employs PatchMerger during training to merge four adjacent patches into one visual token, achieving a 4$\times$ compression. The token reduction ratio (TRR) is defined as the product of the training-aware compression ratio (TACR) and the training-free reduction ratio (TFRR): TRR = TACR $\times$ TFRR.}
    \label{app_tab:qwen2vl}
 
\end{table*}
